# Supplementary material for: Ensemble Kalman filtering with a divided state-space strategy for coupled data assimilation problems
Source: arXiv:1408.4236 ancillary file (2014-08-19)
Supplement: Supplementary file 1 [file supplementary.pdf]

# Supplementary material: A conditional sampling scheme

Suppose that before the update step is applied, the ensemble members of the fast mode are $\{\mathbf{x}_h\}_{h=1}^{n_f}$, while those of the slow mode are $\{\mathbf{z}_h\}_{h=1}^{n_s}$, with $n_f \neq n_s$. Without loss of generality, in what follows we suppose that $n_s < n_f$ and $\{(\mathbf{x}_h, \mathbf{z}_h)\}_{h=1}^{n_s}$ are "matched" pairs in the sense that they are the propagated ensemble members with respect to the "matched" analysis ensemble members at the previous assimilation cycle. Our objective is to generate $(n_f - n_s)$ ensemble members $\{\mathbf{z}_h\}_{h=n_s+1}^{n_f}$ for the slow mode, such that the update formulae can be applied to the ensembles $\{\mathbf{x}_h\}_{h=1}^{n_f}$ and $\{\mathbf{z}_h\}_{h=1}^{n_f}$. The extension of the sampling scheme below to other scenarios is straightforward. For instance, in case that $n_f < n_s$ and one wants to generate $n_s - n_f$ extra ensemble members for the fast mode, then the scheme below can be applied by exchanging the roles of $n_f$ and $n_s$, $\mathbf{x}$ and $\mathbf{z}$, and "fast mode" and "slow mode".

In principle one can draw additional samples by conducting conditional sampling. Let $p(\mathbf{x}, \mathbf{z})$ be the joint probability density function (pdf) of the fast and slow modes, and $p(\mathbf{x})$ the marginal pdf of the fast mode, then the conditional pdf of slow mode is given by $p(\mathbf{z}|\mathbf{x}) = p(\mathbf{x}, \mathbf{z})/p(\mathbf{x})$. In practice, it is often difficult to precisely characterize the state distribution of a nonlinear dynamical model, therefore some approximation, e.g. the Gaussianity assumption, is often made. When Gaussianity is assumed, suppose that the unconditional

mean of the joint state $(\mathbf{x}, \mathbf{z})$ is $(\mu_{\mathbf{x}}, \mu_{\mathbf{z}})$, and the unconditional covariances of $\mathbf{x}$ and $\mathbf{z}$, and their cross-covariance are $\Sigma_{\mathbf{xx}}$, $\Sigma_{\mathbf{zz}}$ and $\Sigma_{\mathbf{xz}}$, respectively, then given a realization, say, $\mathbf{x}_h$ of the fast mode, the conditional mean $\bar{\mu}_{\mathbf{z}}$ and covariance $\bar{\Sigma}_{\mathbf{zz}}$ of the slow mode are (Jazwinski 1970, ch. 2)

$$\bar{\mu}_{\mathbf{z}} = \mu_{\mathbf{z}} + (\Sigma_{\mathbf{xz}})^T (\Sigma_{\mathbf{xx}})^{-1} (\mathbf{x}_h - \mu_{\mathbf{x}}) \, , \tag{1a}$$

$$\bar{\Sigma}_{\mathbf{zz}} = \Sigma_{\mathbf{zz}} - (\Sigma_{\mathbf{xz}})^T (\Sigma_{\mathbf{xx}})^{-1} \Sigma_{\mathbf{xz}} \, . \tag{1b}$$

After $\bar{\mu}_{\mathbf{z}}$ and $\bar{\Sigma}_{\mathbf{zz}}$ are computed, one can draw a sample $\mathbf{z}_h$ from the normal distribution $N(\mathbf{z}; \bar{\mu}_{\mathbf{z}}, \bar{\Sigma}_{\mathbf{zz}})$ to match $\mathbf{x}_h$.

In the context of ensemble data assimilation with large-scale models, two computational issues may arise when evaluating the inverse matrix $(\Sigma_{\mathbf{xx}})^{-1}$ in Eq. (1). One is that, if the ensemble size is less than the dimension of the dynamical model, then $\Sigma_{\mathbf{xx}}$ is singular. In addition, it is often very expensive to compute the inverse of a large matrix. For the above reasons, in the experiment below we do not draw extra samples for the slow mode based on the distribution $N(\mathbf{z}; \bar{\mu}_{\mathbf{z}}, \bar{\Sigma}_{\mathbf{zz}})$. Instead, we do that in a heuristic way. The samples are drawn from the distribution $N(\mathbf{z}; \bar{\mu}_{\mathbf{z}}, \bar{\Sigma}_{\mathbf{zz}})$, where $\bar{\mu}_{\mathbf{z}}$ and $\bar{\Sigma}_{\mathbf{zz}}$ are the sample estimates (based on the background ensemble $\{\mathbf{z}_h\}_{h=1}^{n_s}$) of the unconditional mean $\mu_{\mathbf{z}}$ and covariance $\Sigma_{\mathbf{xx}}$, respectively. Note that, from Eq. (1a) $\bar{\mu}_{\mathbf{z}}$ is a biased estimator of the conditional mean $\bar{\mu}_{\mathbf{z}}$ for a given $\mathbf{x}_h$, but becomes unbiased asymptotically when averaging over different $\mathbf{x}_h$. On the other hand, from Eq. (1b), $\bar{\Sigma}_{\mathbf{zz}}$ tends to over-estimate $\bar{\Sigma}_{\mathbf{zz}}$, and thus introduces certain inflation to the slow mode. In real world applications, extra requirements may also arise in that the generated samples are expected to yield minimal impact on model balance. Readers are referred to, for example, Buehner (2005); Mitchell et al. (2002) and the references therein

for some practical sampling strategies in this aspect.

After sampling, the ensemble members are updated to their analysis counterparts. Then, at the subsequent prediction step, the fast mode propagates $n_f$ ensemble members forward, while the slow mode only integrates $n_s$ members forward. As a result, we randomly single out $n_f - n_s$ ensemble members of the slow mode which will not be propagated forward. For illustration, suppose that it is $\{\mathbf{z}_h\}_{h=n_s+1}^{n_f}$ that are selected out. Then we propagate the matched pairs $\{(\mathbf{x}_h, \mathbf{z}_h)\}_{h=1}^{n_s}$ forward as usual, following the procedures in Fig. 2. On the other hand, the ensemble members $\{\mathbf{z}_h\}_{h=n_s+1}^{n_f}$ of the slow mode are only used as input parameters of the fast mode in order to propagate the members $\{\mathbf{x}_h\}_{h=n_s+1}^{n_f}$ of the fast mode forward to the next assimilation cycle, but not vice versa. That is to say, the members $\{\mathbf{z}_h\}_{h=n_s+1}^{n_f}$ are discarded after the "parametrization", and will not be propagated forward in time.

# REFERENCES


Buehner, M., 2005: Ensemble-derived stationary and flow-dependent background-error covariances: Evaluation in a quasi-operational NWP setting. *Quart. J. Roy. Meteor. Soc.*, **131**, 1013–1043.

Jazwinski, A. H., 1970: *Stochastic Processes and Filtering Theory.* Academic Press, 400 pp.

Mitchell, H. L., P. Houtekamer, and G. Pellerin, 2002: Ensemble size, balance, and model-error representation in an ensemble Kalman filter. *Mon. Wea. Rev.*, **130**, 2791–2808.
